# Supplementary material for: The Competition for Partners in Matching Markets
Source: arXiv:2006.14653 source file (2023-01-11)
Supplement: Supplementary file 1 [file rwoman-concentration-sm.tex]

Within this proof, we assume that $\tau$, $\vec{W}_\tau = \left( W_{j,\tau} \right)_{j \in \mathcal{W}}$, and $\vec{W}_{(n+k)d} = \left( W_{j,(n+k)d} \right)_{j \in \mathcal{W}}$ are revealed (and hence so is $\bar{R}[\tau]$): In what follows, $\mathbb{P}( \cdot )$ and $\mathbb{E}[ \cdot ]$ denote the associated conditional probability and the conditional expectation, respectively.
	
	For brevity, let $w_j \triangleq W_{j,\tau}$, $w_j' \triangleq W_{j,(n+k)d} - W_{j,\tau}$, and $R_j \triangleq \text{Rank}_j( \text{MOSM}(j) )$. %\yk{What is the definition of $R_j$ if woman $j$ is unmatched? It should be degree + 1 if you want the average of $R_j$s to equal $\Rwomen$, right?}
	Note that a woman $j$ receives $w_j$ proposals until time $\tau$ and receives $w_j'$ proposals after time $\tau$ (the total number of proposals $w_j + w_j' = W_{j,(n+k)d}$ equals to her degree).
	Under MOSM, each woman $j$ is matched to her most preferred one among the first $w_j$ proposals, and the rank of her matched partner under MOSM, $R_j$, can be determined by the number of future proposals that she prefers to the matched partner among the remaining $w_j'$ proposals.

\edit{
	More specifically, fix $j$ and let $Y^j_{s,t}$ be the indicator that the woman $j$ prefers her $t^\text{th}$ proposal to her $s^\text{th}$ proposal for $s, t \in \{1, \ldots, w_j+w_j'\}$ with $s \ne t$.
	Then, the rank $R_j$ can be represented as
	\begin{align*}
		R_j &= 1 + \sum_{t=w_j+1}^{w_j+w_j'} \ind\left( \text{woman $j$ prefers her $t^\text{th}$ proposal to all of her first $w_j$ proposals} \right) 
			\\&= 1 + \sum_{t=w_j+1}^{w_j+w_j'} \prod_{s=1}^{w_j} \ind\left( \text{woman $j$ prefers her $t^\text{th}$ proposal to her $s^\text{th}$ proposal} \right) 
			\\&= 1 + \sum_{t=w_j+1}^{w_j+w_j'} \prod_{s=1}^{w_j} Y^j_{s,t}, \,
	\end{align*}
	where we define $\prod_{s=1}^{w_j} \cdot = 1$ if $w_j = 0$ for convenience.
	Observe that $\{ Y^j_{s,t} \}_{s,t}$ are negatively associated (NA) by Lemma \ref{lem:NA}-\eqref{lem:NA-permutation} since  $( Y^j_{s,t} )_{s,t \in \{1, \ldots, w_j+w_j'\}, s \ne t }$ is a uniformly random permutation of $\frac{ (w_j+w_j')(w_j+w_j'-1) }{2}$ ones and $\frac{ (w_j+w_j')(w_j+w_j'-1) }{2}$ zeros due to symmetry.
	\sm{May not be true}
	Consequently, $\prod_{s=1}^{w_j} Y^j_{s,t}$ is a component-wise increasing function of $Y^j_{1,t}, \ldots, Y^j_{w_j,t}$ and hence $\{ \prod_{s=1}^{w_j} Y^j_{s,t} \}_{t \in \{w_j+1, \ldots, w_j+w_j'\}}$ are also NA by Lemma \ref{lem:NA}-\eqref{lem:NA-monotone}.
	Also note that $\prod_{s=1}^{w_j} Y^j_{s,t} \sim \text{Bernoulli}\left( \frac{1}{w_j+1} \right)$ for each $t$.
	Therefore,
	\begin{equation*}
		\mathbb{E}\left[ R_j \right] = 1 + \frac{w_j'}{w_j+1},
	\end{equation*}
	and, for any $\lambda \in \mathbb{R}$, we have
	\begin{align*}
		\mathbb{E}\left[ \exp\left( \lambda (R_j-1) \right) \right]
			&\leq \prod_{t=w_j}^{w_j + w_j'} \mathbb{E}\left[ \exp\left( \lambda \prod_{s=1}^{w_j} Y^j_{s,t} \right) \right]
			= \left( 1 - \frac{1}{w_j+1} + \frac{1}{w_j+1} e^\lambda \right)^{w_j'}
			\\&\leq \exp\left( \frac{1}{w_j+1} \left(e^\lambda -1\right) \right)^{w_j'}
			= \exp\left( \frac{w_j'}{w_j+1} \left(e^\lambda -1\right) \right),
	\end{align*}
	where we utilized the fact that $\left\{ \exp\left( \lambda \prod_{s=1}^{w_j} Y^j_{s,t} \right) \right\}_{t \in \{w_j+1, \ldots, w_j+w_j'\}}$ are NA and that $1-x \leq e^{-x}$ for any $x \in \mathbb{R}$.
}
	
\edit{
	Further observe that $R_j$'s are independent across $j$ (conditioned on $\vec{W}_\tau$ and $\vec{W}_{(n+k)d}$).
	Therefore, for any $\lambda \in \mathbb{R}$, we obtain
	\begin{align*}
		\mathbb{E}\left[ \exp\left( \lambda \sum_{j \in \mathcal{W}} (R_j - 1) \right) \right]
			&= \prod_{j \in \mathcal{W}} \mathbb{E}\left[ \exp\left( \lambda (R_j-1) \right) \right]
			\leq \prod_{j \in \mathcal{W}} \exp\left( \frac{w_j'}{w_j+1} \left( e^\lambda -1 \right) \right)
			\\&= \exp\left( \sum_{j \in \mathcal{W}} \frac{w_j'}{w_j+1} \left( e^\lambda -1 \right) \right) 
			= \exp\left( n \bar{R}[\tau] (e^\lambda-1) \right),
	\end{align*}
	since $\bar{R}[\tau] = \frac{1}{n} \sum_{j \in \mathcal{W}} \frac{w_j'}{w_j+1}$ by its definition.
}

	\begin{equation*}
		R_j = 1 + \sum_{s=w_j+1}^{w_j+w_j'} X_{j,s}
	\end{equation*}
	where $X_{j,s}$ is defined as the indicator that woman $j$ prefers her $s^\text{th}$ incoming proposal (after termination of DA) to her partner under MOSM.
	Observe that $X_{j,s} \sim \text{Bernoulli}\left( \frac{1}{w_j+1} \right)$ and is independent across $j$ and $s$. \yk{I don't think it's independent! If the first three proposals are better than her partner, it becomes more likely her partner is shitty and hence the fourth proposal is more likely to also be better than her partner.. If you agree, then that breaks the claim it is Binomial below and stuff after that. However, I think you can nevertheless use Hoeffding's inequality to show that 
$$\mathbb{P}\left( \left. \Wrank \geq 1 + (1+\epsilon) \bar{R}[\tau] \,\right| \vec{W}_\tau, \vec{W}_{(n+k)d}\right) \leq 
\exp \left ( -\frac{2\eps^2  \bar{R}[\tau]^2 n^2 }{\sum_{j \in \mathcal{W}}W_{j,(n+k)d}^2 } \right )
$$. This should suffice since (i) you already showed that wvhp $\bar{R}[\tau] \geq \sqrt{d}/2$ and (ii) you can also show, using negative association that $\sum_{j \in \mathcal{W}}W_{j,(n+k)d}^2 / n$ is no more than $2d^2$ wvhp. Overall, the RHS should be less than $\exp(-n^{1-\epsilon})$ wvhp, which should suffice for your purposes, no?
} \edit{It follows from $X_{j,s} \sim \text{Bernoulli}\left( \frac{1}{w_j+1} \right)$ that the conditional expectation of $R_j = 1+ \frac{w_j'}{w_j+1}$ and hence that the conditional expectation of $\Wrank$ is $1+\bar{R}[\tau]$, which proves the first sentence of the lemma.}
	Therefore,
	\begin{equation*}
		-1 + R_j \stackrel{\text{d}}{=} \text{Binomial}\left( w_j', \frac{1}{w_j+1} \right),
	\end{equation*}
	and $R_j$'s are independent across $j$. \yk{I agree that $R_j$'s are independent across $j$.}
	Consequently, for any $\lambda \in \mathbb{R}$,
	\begin{align*}
		\mathbb{E}\left[ \exp\left( \lambda \sum_{j \in \mathcal{W}} (R_j - 1) \right) \right]
			&= \prod_{j \in \mathcal{W}} \left( 1 - \frac{1}{w_j+1} + \frac{1}{w_j+1} e^\lambda \right)^{w_j'}
			\leq \prod_{j \in \mathcal{W}} \exp\left( \frac{1}{w_j+1} (e^\lambda-1) \right)^{w_j'}
			\\&= \prod_{j \in \mathcal{W}} \exp\left( \frac{w_j'}{w_j+1} (e^\lambda-1) \right)
			= \exp\left( n \bar{R}[\tau] (e^\lambda-1) \right),
	\end{align*}
	since $\bar{R}[\tau] = \frac{1}{n} \sum_{j \in \mathcal{W}} \frac{w_j'}{w_j+1}$ by its definition.

	By Markov's inequality, for any $\lambda \in [0,1]$,
	\begin{align*}
		\mathbb{P}\left( -1 + \frac{1}{n} \sum_{j \in \mathcal{W}} R_j \geq (1+\epsilon) \bar{R}[\tau] \right)
			&\leq \frac{ \mathbb{E}\left[ \exp\left( \lambda \sum_{j \in \mathcal{W}} (R_j-1) \right) \right] }{ \exp\left( n \bar{R}[\tau] \lambda(1+\epsilon)  \right) }
			\\&\leq \exp\left(  n \bar{R}[\tau] (e^\lambda-1) - n \bar{R}[\tau] \lambda (1+\epsilon)   \right)
			\\&\leq \exp\left(  n \bar{R}[\tau] (\lambda + \lambda^2) - n \bar{R}[\tau] \lambda (1+\epsilon)   \right)
			= \exp\left( n \bar{R}[\tau] (\lambda^2 - \lambda \epsilon) \right),
	\end{align*}
	where we use the fact that $e^x \leq 1 + x + x^2$ for $x \leq 1$.
	By setting $\lambda \triangleq \frac{\epsilon}{2}$, we obtain
	\begin{align*}
		\mathbb{P}\left( \frac{1}{n} \sum_{j \in \mathcal{W}} R_j \geq 1 + (1+\epsilon) \bar{R}[\tau] \right) \leq \exp\left( - \frac{1}{4} \epsilon^2 n \bar{R}[\tau] \right).
	\end{align*}
